# Supplementary material for: EMATO: Energy-Model-Aware Trajectory Optimization for Autonomous Driving
Source: arXiv:2412.08830 source file (2024-12-12)
Supplement: Supplementary file 1 [file appendix.tex]

\subsection{Appendix}

\begin{table}[h]
\caption{Vehicle Parameters}
\centering % Center the table within the text block
\begin{tabular}{c|c|c||c|c|c} % Define a table with 5 columns
\hline
\textbf{Param} & \textbf{Sedan} & \textbf{Truck} & \textbf{Param} & \textbf{Sedan} & \textbf{Truck}\\
\hline
$M$   & 1200 & 4800 & $o_1$ & 1.0254e-2 & 9.0901e-3 \\
$A_v$  &  2.5  & 2.5 & $o_2$ & -9.2812e-4 & 3.7574e-8 \\
$\rho$   & 1.184 & 1.184 &$o_3$  & 2.154e-5 & 3.4935e-8 \\
$C_d$   & 0.32 & 0.6 & $o_4$  & -4.2427e-7 & 2.4230e-4 \\  
$\mu$  & 0.015  & 0.006 & $c_0$ &  0.07224 & 1.6550e-1           \\
$g$     & 9.81 & 9.81   &  $c_1$ & 0.09681 & 3.6070e-1              \\
$o_0$ &  1.4627e-1 &3.351e-1 & $c_2$ & 1.0750e-3 &  2.4223e-4       \\
\hline
\end{tabular}
\label{tab_vehicle_parameters}
\end{table}

\begin{table}[h]
\caption{Dynamics Parameters}
\centering % Center the table within the text block
\begin{tabular}{c|c|c} % Define a table with 3 columns
\hline
\textbf{Param} & \textbf{Sedan} & \textbf{Truck} \\
\hline
$v_{\text{max}}$ & 27 (m/s) & 27  \\
${a_v}_{\text{max}}$ & 2.0 & 2.0 \\
${a_b}_{\text{max}}$ & 5.0 & 5.0 \\
$ {a_t}_{\text{max}}$ & 3.0 & 3.0 \\
$j_{\text{max}}$ & 10.0 & 5.0 \\
\hline
\end{tabular}
\label{tab_vehicle_parameters}
\end{table}

\begin{table}[h]
\caption{ACC Parameters}
\centering % Center the table within the text block
\begin{tabular}{c|c} % Define a table with 3 columns
\hline
\textbf{Param} & \textbf{Value}  \\
\hline
$T_h$ & 1.5 \\
$\Delta l_s $ & 50 \\
$\Delta l _{\text{max}}$ & 300 \\
$ \Delta l_r$ & 10 \\
\textit{EMATO-V} \textbf{w} & [0.01,14.51,14.51,1.16,38.91] \\
\textit{EMATO-B} \textbf{w} & [0,14.51,14.51,1.16,38.91] \\
\textit{EMATO-R} \textbf{w} & [0,14.51,14.51,1.16,38.91] \\
\hline
\end{tabular}
\label{tab_vehicle_parameters}
\end{table}

\begin{table}[h]
\caption{Frenet Parameters}
\centering % Center the table within the text block
\begin{tabular}{c|c} % Define a table with 3 columns
\hline
\textbf{Param} & \textbf{Value}  \\
\hline
$v_d$ for \textit{QF-V} & 70 (km/h) = 19.44 (m/s) \\
\textit{QF-V} \textbf{w} & [1,0,0,0,0] \\
\textit{QF-M} \textbf{w} & [1,0,0,0.001,100] \\
\textit{QF-E} \textbf{w} & [0,0,0,0,1] \\
\textit{EMATO-FV} \textbf{w} & [0,14.51,14.51,1.16,38.91] \\
\textit{EMATO-FM} \textbf{w} & [0,14.51,14.51,1.16,38.91] \\
\textit{EMATO-FE} \textbf{w} & [0,14.51,14.51,1.16,38.91] \\
\hline
\end{tabular}
\label{tab_vehicle_parameters}
\end{table}
